# Supplementary material for: Coherent Modulation of Quasiparticle Scattering Rates in a Photoexcited Charge-Density-Wave System
Source: arXiv:2108.12323 ancillary file (2022-01-04)
Supplement: Supplementary file 1 [file Supplemental_material.pdf]

# Coherent Modulation of Quasiparticle Scattering Rates in a Photoexcited Charge-Density-Wave System

## *Supplemental Material*

J. Maklar<sup>1</sup>, M. Schüler<sup>2</sup>, Y. W. Windsor<sup>1</sup>, C. W. Nicholson<sup>1</sup>, M. Puppin<sup>1</sup>, P. Walmsley<sup>2,3</sup>,  
I. R. Fisher<sup>2,3</sup>, M. Wolf<sup>1</sup>, R. Ernstorfer<sup>1,4</sup>, M. A. Sentef<sup>5</sup>, L. Rettig<sup>1</sup>

<sup>1</sup>Fritz-Haber-Institut der Max-Planck-Gesellschaft, Faradayweg 4-6, 14195 Berlin, Germany

<sup>2</sup>Stanford Institute for Materials and Energy Sciences (SIMES), SLAC National Accelerator Laboratory, Menlo Park, CA 94025, USA

<sup>3</sup>Geballe Laboratory for Advanced Materials and Department of Applied Physics, Stanford University, CA 94305, USA

<sup>4</sup>Institut für Optik und Atomare Physik, Technische Universität Berlin, Straße des 17. Juni 135, 10623 Berlin, Germany

<sup>5</sup>Max Planck Institute for the Structure and Dynamics of Matter, Luruper Chaussee 149, 22761 Hamburg, Germany

August 11, 2021

## 1 Estimation of the experimental charge-density-wave gap

To determine the experimental transient charge-density-wave (CDW) energy gap  $\Delta_{\text{CDW}}$  near the Fermi level  $E_{\text{F}}$ , we first extract the energy distribution curves (EDCs) of the gapped momentum region, indicated in Main Fig. 2(b), for different pump-probe delays. Next, we fit the individual EDCs using two Gaussians to describe the peaks below and above  $E_{\text{F}}$ , respectively. To account for the time-dependent occupation of electronic states due to a transiently varying electronic temperature upon optical excitation, the Gaussians are multiplied by a Fermi-Dirac distribution. The resulting fit function is given by

$$I(E) = \left( A_1 \exp\left(-\frac{(E - E_1)^2}{2\sigma_1^2}\right) + A_2 \exp\left(-\frac{(E - E_2)^2}{2\sigma_2^2}\right) \right) \cdot \frac{1}{\exp(E - E_{\text{F}}/k_{\text{B}}T_{\text{e}}) + 1} \quad (1)$$

with Gaussian amplitude  $A_{1/2}$ , peak position  $E_{1/2}$ , variance  $\sigma_{1/2}^2$ , transient electronic temperature  $T_{\text{e}}$  and Boltzmann constant  $k_{\text{B}}$ . The transient electronic temperature  $T_{\text{e}}$ , see Fig. S1, and Fermi level  $E_{\text{F}}$ , which enter the fit function as fixed parameters, are extracted from the metallic part of the Fermi surface, as discussed in detail in Ref. [1]. The Gaussian amplitudes, peak positions and variances are kept as free fit parameters. This model yields an excellent description of the experimental EDCs for time delays, at

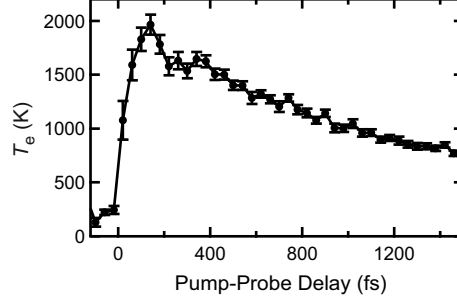

Figure S1: Transient electronic temperature  $T_e$  with one standard deviation as uncertainty extracted from the metallic part of the Fermi surface using a Fermi-Dirac fit.

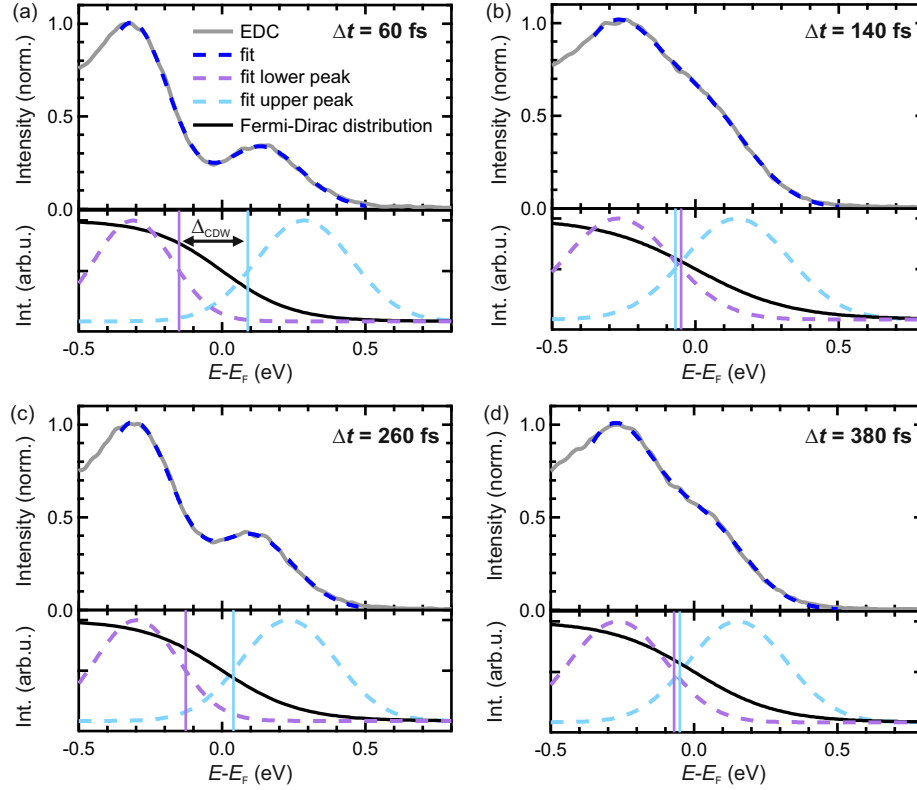

Figure S2: (a-d) Top: EDCs extracted from the momentum region featuring the CDW energy gap (indicated in Main Fig. 2b) for selected pump-probe delays with best fits using Eq. 1. Bottom: Individual components of the best fits (lower/upper Gaussian peak and Fermi-Dirac distribution). The intensities of the individual curves have been rescaled for clarity. Note that the apparent shift of the central positions of the individual Gaussians with respect to the total fit function is caused by the multiplication with the Fermi-Dirac distribution. The purple/blue solid lines mark the midpoint energies of the leading/trailing edges used to approximate  $\Delta_{\text{CDW}}$ .

which the relevant states above  $E_F$  are populated ( $0 \text{ fs} < \Delta t < 1000 \text{ fs}$ ). Exemplary fits are shown in Fig. S2.

Finally, we approximate the size of  $\Delta_{\text{CDW}}$  using the difference of the midpoint energies of the leading/trailing edges of the lower/upper peaks, as depicted in Fig. S2. The midpoint energies of the respective edges can be expressed as a shift by the half width at half maximum from the central Gaussian peak positions, with Gaussian 1 describing the peak below and Gaussian 2 the peak above  $E_F$ :

$$\Delta_{\text{CDW}} = \left( E_2 - \frac{2\sqrt{2 \ln 2} \sigma_2}{2} \right) - \left( E_1 + \frac{2\sqrt{2 \ln 2} \sigma_1}{2} \right) \quad (2)$$

This edge midpoint approach is a common and reliable method in ARPES to estimate the size of energy gaps, as, e.g., demonstrated for various superconductors [2–4]. The reliability of this approach is further supported by the fact that the initial CDW energy gap near  $\Delta t \sim 0 \text{ fs}$  is in excellent agreement with previous studies (400 meV [5]).

To determine the uncertainty of  $\Delta_{\text{CDW}}$ , we sum the individual uncertainties of the parameters entering the edge midpoint approach (Eq. 2). To account for the uncertainty of  $T_e$  and  $E_F$  entering the initial fit function as constant coefficients (Eq. 1), we calculated the standard deviation of  $\Delta_{\text{CDW}}$  obtained from one thousand successive EDC fits with coefficients  $T_e$  and  $E_F$  varied randomly around their center values with a normally distributed probability of width  $\sigma_{T_e}$  and  $\sigma_{E_F}$ , respectively. The resulting mean values of  $\Delta_{\text{CDW}}$  with one standard deviation as uncertainty for different pump-probe delays  $\Delta t$  are shown in Fig. S3(a). Note that the large error of  $\Delta_{\text{CDW}}$  near  $\Delta t \sim 0 \text{ fs}$  results from the fact that the electrons have not fully reached a thermal distribution yet, leading to a large uncertainty of the electronic temperature.

## 2 Determination of the experimental transient lifetimes

To model the transient population intensities, we first extract the transient size of the CDW energy gap upon photoexcitation. We describe the CDW gap dynamics using an exponentially damped, absolute sinusoidal fit function with a frequency change over time (chirp) and a linear background with slope  $a$ , which is convolved with a Gaussian (FWHM=35 fs) to account for the temporal resolution of the experiment:

$$\Delta_{\text{CDW}}(\Delta t) = \left( \Delta_0 \cdot \exp(-\Delta t / \tau_{\text{damp}}) \cdot \left| \sin \left( 2\pi \Delta t (f + f_{\text{chirp}} \cdot \Delta t) + \phi \right) \right| + a\Delta t \right) * \text{Gaussian} \quad (3)$$

This allows for an excellent description of the experimental data, see Fig. S3(a). The resulting best fit coefficients, i.e., the decay constant of the oscillation amplitude  $\tau_{\text{damp}} = 450 \text{ fs}$ , the oscillation frequency  $f = 2.23 \text{ THz}$ , the frequency chirp  $f_{\text{chirp}} = -0.36 \text{ THz/ps}$ , and phase  $\phi = 0.39 \pi$ , are subsequently used for modeling the transient photoemission intensities.

To describe the transient intensities in the regions of interest (ROIs) 1 and 2 of Main Fig. 2a, we employ a single-exponential decay with amplitude  $A$  and lifetime  $\tau_{\text{exp}}$ , convolved with a Gaussian (FWHM=35 fs):

$$I(\Delta t) = A \cdot \exp(-\Delta t / \tau_{\text{exp}}(\Delta t)) * \text{Gaussian} \quad (4)$$

However, a bare exponential decay with constant lifetime can not reproduce the experimental data, as the photoemission intensities feature a transient modulation of the relaxation rates. These deviations from a single-exponential decay are further emphasized by the derivatives of the transient photoemission intensities with respect to  $\Delta t$ , as shown in Fig. S3(b)–(c), which feature distinct modulations that coincide with the collective CDW dynamics. Whenever the CDW gap at  $E_F$  opens, see Fig. S3(a), the relaxation of the high-energy population slows down, indicated by the local minimum of the derivative  $|dI/d\Delta t|$ . Conversely, when the system reaches the metallic state corresponding to  $\Delta_{\text{CDW}} \sim 0$  eV, the high-energy population relaxes faster, indicated by a local maximum of  $|dI/d\Delta t|$ .

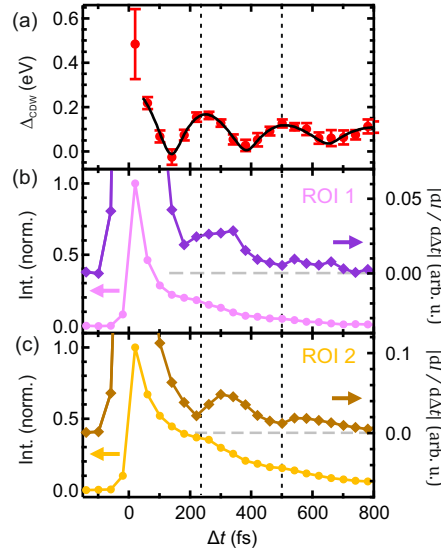

Figure S3: (a) Extracted transient CDW energy gap with one standard deviation as uncertainty. The black solid line marks the best fit using a chirped sinusoidal function (Eq. 3). (b-c) Photoemission intensities versus  $\Delta t$  from the ROIs indicated in Main Fig. 2(a). The derivatives of the photoemission intensities with respect to  $\Delta t$  (purple/brown, right axis, absolute values, numerical differentiation by central differences) emphasize the deviation from an exponential decay with constant lifetime, as they feature distinct modulations that coincide with the oscillations of  $\Delta_{\text{CDW}}$ . The dashed lines serve as guides to the eye.

To account for this oscillatory component of the carrier relaxation rate, we employ a time-dependent lifetime based on the previously extracted parameters of the CDW gap dynamics:

$$\tau_{\text{exp}}(\Delta t) = \tau_{\text{metal}} + \tau_{\text{CDW}} \cdot \exp(-\Delta t/\tau_{\text{damp}}) \cdot \left| \sin \left( 2\pi \Delta t (f + f_{\text{chirp}} \cdot \Delta t) + \phi \right) \right| \quad (5)$$

This phenomenological description of the total lifetime comprises the lifetime of the metallic state,  $\tau_{\text{metal}}$ , which serves as a baseline, on top of which an exponentially damped, oscillatory contribution with amplitude  $\tau_{\text{CDW}}$ , corresponding to the observed transient lifetime increase in the CDW state, is added. The functional form of the sine with frequency  $f$ , chirp  $f_{\text{chirp}}$ , the phase offset  $\phi$ , and a damping prefactor with lifetime  $\tau_{\text{damp}}$ , allows us to incorporate the observed dynamics of the CDW gap size  $\Delta_{\text{CDW}}$  into the total lifetime  $\tau_{\text{exp}}$ . We fit the transient photoemission intensities (ROIs 1 and 2) using Eqs. 4 and 5, keeping only  $\tau_{\text{metal}}$ ,  $\tau_{\text{CDW}}$  and the amplitude  $A$  as variable fit parameters, while keeping the remaining parameters

(extracted from the transient CDW gap fit) fixed. This approach yields an excellent description of the experimental data, see Main Fig. 2(e)–(f). The resulting fit coefficients are summarized in Supplementary Table 1.

Finally, this allows us to investigate the dependency of the experimental transient lifetime  $\tau_{\text{exp}}(\Delta t)$  as a function of the extracted CDW gap size  $\Delta_{\text{CDW}}(\Delta t)$  and a comparison to the theoretical simulations with a static CDW gap, as displayed in Main Fig. 3(c) for ROI 1. The transient lifetime  $\tau_{\text{exp}}(\Delta t)$  determined from ROI 2 versus  $\Delta_{\text{CDW}}(\Delta t)$  is shown in Fig. S4, which follows a similar trend.

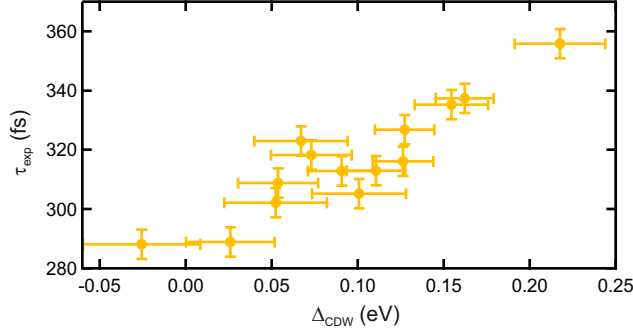

Figure S4: Transient lifetimes  $\tau_{\text{exp}}(\Delta t)$  from Main Fig. 2(f), ROI 2, versus the experimentally extracted  $\Delta_{\text{CDW}}(\Delta t)$ . The error bars correspond to one standard deviation of the respective fits of  $\tau_{\text{exp}}$  and  $\Delta_{\text{CDW}}$ .

Table 1: Best fit coefficients of the decay fits displayed in Main Fig. 2(e)–(f).

| Variable              | Physical meaning                         | fixed or free | ROI 1 | ROI 2 | unit   |
|-----------------------|------------------------------------------|---------------|-------|-------|--------|
| $A$                   | amplitude                                | free          | 0.48  | 0.67  |        |
| $\tau_{\text{metal}}$ | lifetime of metallic phase               | free          | 160   | 287   | fs     |
| $\tau_{\text{CDW}}$   | lifetime contribution of CDW phase       | free          | 96    | 91    | fs     |
| $\tau_{\text{damp}}$  | damping prefactor of $\tau_{\text{CDW}}$ | fixed         | 450   | 450   | fs     |
| $f$                   | oscillation frequency                    | fixed         | 2.23  | 2.23  | THz    |
| $f_{\text{chirp}}$    | frequency chirp                          | fixed         | -0.36 | -0.36 | THz/ps |
| $\phi$                | phase offset                             | fixed         | 0.39  | 0.39  | $\pi$  |

### 3 Details on the simulations

#### 3.1 Tight-binding model

For the simulations we employ the tight-binding (TB) model from Ref. [6] for the quasi-2D Te planes, including the  $p_x$  and  $p_z$  orbitals. In absence of any CDW order, the Hamiltonian is defined by

$$\mathbf{h}(\mathbf{k}) = \begin{bmatrix} \varepsilon_x(\mathbf{k}) & V_{xz} \\ V_{xz} & \varepsilon_z(\mathbf{k}) \end{bmatrix}, \quad (6)$$

where

$$\begin{aligned} \varepsilon_x(\mathbf{k}) &= -2t_{\parallel} \cos\left[\frac{1}{2}(k_x + k_z)a\right] - 2t_{\perp} \cos\left[\frac{1}{2}(k_x - k_z)a\right] \\ \varepsilon_z(\mathbf{k}) &= -2t_{\parallel} \cos\left[\frac{1}{2}(k_x - k_z)a\right] - 2t_{\perp} \cos\left[\frac{1}{2}(k_x + k_z)a\right]. \end{aligned}$$

The hybridization between the  $p_x$  and  $p_z$  bands is determined by  $V_{xz}$ . For the lattice constants we approximate  $a \approx c$ . All calculations are performed in the extended 2D Brillouin zone (instead of the reduced 3D Brillouin zone). We will use the labels  $m, m' \in \{p_x, p_z\}$  for the orbitals.

Following Ref. [6], the incommensurate CDW with wave-vector  $\mathbf{q}_{\text{CDW}}$  can be described by expanding the Hamiltonian (6) in terms of harmonics of  $\mathbf{q}_{\text{CDW}}$ . Due to the weak intensity of the observed shadow bands, truncating after the first harmonic yields an accurate description. Accordingly the extended Hamiltonian reads

$$\tilde{\mathbf{h}}(\mathbf{k}) = \begin{bmatrix} \mathbf{h}(\mathbf{k} - \mathbf{q}_{\text{CDW}}) & \mathbf{V} & 0 \\ \mathbf{V} & \mathbf{h}(\mathbf{k}) & \mathbf{V} \\ 0 & \mathbf{V} & \mathbf{h}(\mathbf{k} + \mathbf{q}_{\text{CDW}}) \end{bmatrix}. \quad (7)$$

For simplicity we chose the coupling  $\mathbf{V} = V_{\text{CDW}}\mathbf{I}$ . The parameter  $V_{\text{CDW}}$  determines the size of the gap and the intensity of the shadow bands. We chose  $t_{\parallel} = 1.7$  eV,  $t_{\perp} = 0.32$  eV, and  $V_{xz} = 0.2$  eV, which best matches the experimental band structure. The coupling strength  $V_{\text{CDW}}$  is treated as a parameter.

#### 3.2 Many-body treatment

To obtain a realistic model that includes generic electron-electron (e-e) scattering, we consider the Hubbard model with identical on-site repulsion  $U$  for each orbital. For convenience we combine the orbital and the CDW index into a single index  $i = (m, N)$  where  $N = -1, 0, 1$  denotes the sectors in Eq. (7). We consider the many-body Hamiltonian

$$\hat{H} = \hat{H}_0 + \hat{H}_{\text{e-e}} \equiv \sum_{\mathbf{k}} \sum_{ij, \sigma} \tilde{h}_{ij}(\mathbf{k}) \hat{c}_{\mathbf{k}i\sigma}^{\dagger} \hat{c}_{\mathbf{k}j\sigma} + U \sum_{\mathbf{k}, \mathbf{p}, \mathbf{q}} \sum_{ij, \sigma} \hat{c}_{\mathbf{k}+\mathbf{q}i\sigma}^{\dagger} \hat{c}_{\mathbf{p}-\mathbf{q}j\sigma}^{\dagger} \hat{c}_{\mathbf{p}j\sigma} \hat{c}_{\mathbf{k}i\sigma}. \quad (8)$$

Note that the interaction term in Eq. (8) entails an additional simplification, as some combinations of sectors (with respect to Eq. (7)) are excluded. This assumption is justified by the following: (i) scattering processes with small momentum transfer dominate in the experimentally relevant bands (this is particularly pronounced in the more realistic case of a long-range Coulomb interaction); (ii) coupling of different sectors is very weak except for close to the gap region.

To capture the dynamics in presence of e-e interactions, we employ the time-dependent nonequilibrium Green's functions (td-NEGF) framework. To this end we consider the Green's function (GF) on the Kadanoff-Baym contour  $\mathcal{C}$  [7],

$$G_{ij\sigma}(\mathbf{k}; t, t') = -i \langle T_{\mathcal{C}} \hat{c}_{\mathbf{k}i\sigma}(t) \hat{c}_{\mathbf{k}j\sigma}^{\dagger}(t') \rangle . \quad (9)$$

Here,  $T_{\mathcal{C}}$  denotes the contour ordering symbol. The contour GF (9) contains information on the photoemission spectrum when choosing the location of the contour arguments  $t, t'$  accordingly. In particular, the time-resolved photoemission intensity is obtained by the lesser GF  $G_{ij\sigma}^<(\mathbf{k}; t, t') = i \langle \hat{c}_{\mathbf{k}j\sigma}^{\dagger}(t') \hat{c}_{\mathbf{k}i\sigma}(t) \rangle$  by [8, 9]

$$I(\mathbf{k}, \omega, \Delta t) \propto \text{Im} \sum_{m,\sigma} \int dt \int dt' s(t) s(t') e^{i\omega(t-t')} G_{(m0)(m0)\sigma}^<(\mathbf{k}; t, t') . \quad (10)$$

Here we have projected onto the first Brillouin zone containing the main bands (middle sector in Eq. (7)). The energy  $\omega$  corresponds to the binding energy, while  $s(t)$  denotes the shape of the probe pulse, which is delayed with respect to the pump pulse by  $\Delta t$ .

The GF (9) is obtained by solving its equation of motion

$$\left( i\partial_t - \tilde{\mathbf{h}}(\mathbf{k}, t) \right) \mathbf{G}(\mathbf{k}; t, t') + \int_{\mathcal{C}} d\bar{t} \mathbf{\Sigma}(\mathbf{k}; t, \bar{t}) \mathbf{G}(\mathbf{k}; \bar{t}, t') , \quad (11)$$

where we have employed the compact matrix notation. The self-energy  $\mathbf{\Sigma}(\mathbf{k}; t, t')$  captures the many-body effects arising due to e-e scattering. The pump pulse is incorporated by the Peierl's substitution  $\tilde{\mathbf{h}}(\mathbf{k}, t) = \tilde{\mathbf{h}}(\mathbf{k} - q\mathbf{A}(t))$ , where  $\mathbf{A}(t)$  stands for the vector potential of the pulse.

Solving the full Kadanoff-Baym equations (11) is a tremendous computational challenge for the resolution with respect to momentum space and reaching relevant time scales. Therefore we employ the generalized Kadanoff-Baym ansatz (GKBA), which transform Eq. (11) into an equation of motion for the single-particle density matrix  $\rho(\mathbf{k}, t)$ :

$$\frac{d}{dt} \rho(\mathbf{k}, t) + i[\tilde{\mathbf{h}}(\mathbf{k}, t), \rho(\mathbf{k}, t)] = -(\mathbf{I}(\mathbf{k}, t) + \text{h. c.}) . \quad (12)$$

The quasi-particle scattering effects captured by the self-energy enter the dynamics of the density matrix (12) via the collision integral

$$\mathbf{I}(\mathbf{k}, t) = \int_{-\infty}^t d\bar{t} \left( \mathbf{\Sigma}^<(\mathbf{k}; t, \bar{t}) \mathbf{G}^{\text{A}}(\mathbf{k}; \bar{t}, t) + \mathbf{\Sigma}^{\text{R}}(\mathbf{k}; t, \bar{t}) \mathbf{G}^<(\mathbf{k}; \bar{t}, t) \right) . \quad (13)$$

Following the same route as in Ref. [10], the correlated equilibrium density matrix  $\rho(\mathbf{k}, t)$  is obtained from adiabatically switching on the interactions. Extensive benchmarks [10–13] underpin the accuracy of the GKBA in the relevant regime of weak to moderate interactions.

Eq. (12) is solved with a highly accurate computer code (more details in Ref. [10]). A  $N_k = 72 \times 72$  sampling of the Brillouin zone was used, while the time propagation was done in equidistant steps of  $h = 0.8$  a.u. and up to  $N_t = 7500$  time steps. After obtaining  $\rho(\mathbf{k}, t)$  the lesser GF is reconstructed by

$$\mathbf{G}^<(\mathbf{k}; t, t') = \mathbf{G}^{\text{R}}(\mathbf{k}; t, t') \rho(\mathbf{k}, t') + \rho(\mathbf{k}, t) \mathbf{G}^{\text{A}}(\mathbf{k}; t, t') . \quad (14)$$

The retarded (advanced) GF  $\mathbf{G}^{\text{R}}(\mathbf{k}; t, t')$  ( $\mathbf{G}^{\text{A}}(\mathbf{k}; t, t')$ ) is defined with respect to the mean-field Hamiltonian. Substituting the lesser GF (14) into Eq. (10) then yields the time-resolved photomission spectra.

### 3.3 Calculation of the self-energy

The sharply defined bands in the experimental ARPES data and the unusually long lifetime of excited electrons indicate a weak-coupling scenario, in which the e–e interaction can be treated perturbatively. Thus, we employ the second-Born approximation, which defines the self-energy as

$$\Sigma_{ij}^{e-e,\gtrless}(\mathbf{k}; t, t') = i \frac{U^2}{N_k} \sum_{\mathbf{q}} G_{ij}^{\gtrless}(\mathbf{k} - \mathbf{q}; t, t') P_{ij}^{\gtrless}(\mathbf{q}; t, t'), \quad (15)$$

where

$$P_{ij}^{\gtrless}(\mathbf{q}; t, t') = -\frac{2i}{N_k} \sum_{\mathbf{p}} G_{ij}^{\gtrless}(\mathbf{q} + \mathbf{p}; t, t') G_{ji}^{\lessgtr}(\mathbf{p}; t', t) \quad (16)$$

denotes the electron-hole polarization. For brevity we have dropped the spin index, as all quantities are spin-independent. Eq. (15)–(16) are evaluated numerically and inserted into the collision integral (13). For a qualitative analysis we have also computed the polarization (16) for the equilibrium state, inserting the non-interacting GF. Specifically we calculate the retarded component

$$P_{ij}^{(0),R}(\mathbf{q}; \omega) = \int_0^\infty dt e^{i\omega t} \left[ P_{ij}^{(0),>}(\mathbf{q}; t, 0) - P_{ij}^{(0),<}(\mathbf{q}; t, 0) \right], \quad (17)$$

where the superscript (0) indicates the free GFs entering the definition. For the practical evaluation of the one-shot polarization (17) we insert the time-dependent GFs and perform the integration analytically. Note that a considerably more dense sampling of the Brillouin zone is required to achieve convergence in the real-frequency representation. We include up to  $N_k = 300 \times 300$  points to ensure converged results. The average polarization  $\bar{P}^R(\omega)$  presented in Fig. 4(d) in the main text is computed from Eq. (17) by

$$\bar{P}^R(\omega) = \frac{1}{\pi q_c^2} \sum_m \int_{|\mathbf{q}| < q_c} d\mathbf{q} P_{(m0)(m0)}^{(0),R}(\mathbf{q}; \omega), \quad (18)$$

where  $q_c = 0.05$  a.u. is a typical value for the scattering processes with small momentum transfer.

## 4 Simulation of the relaxation dynamics

We have performed simulations within the GKBA formalism to discern the scattering channels and explain the slow-down of the relaxation dynamics observed in the experiments. The calculations are agnostic with respect to the origin of the CDW; we focus on the dynamics of highly excited carriers. As the variation of the photoemission intensity in the gap region – the hallmark of the collective CDW excitation – is slow on the electronic time scale, we keep the CDW frozen in the simulations.

The dynamics is triggered by a short laser pulse, described by the vector potential

$$\mathbf{A}(t) = \mathbf{e} A_0 \sin[\omega_0(t - t_0)] \sin^2\left(\frac{\pi(t - t_0)}{T_p}\right), \quad t_0 < t < t_0 + T_p, \quad (19)$$

where  $\mathbf{e}$  is the polarization vector,  $\omega_0$  the central frequency, and  $T_p = 2\pi n_c / \omega_0$  the duration of a  $n_c$ -cycle pulse. We fix  $\omega_0 = 1.5$  eV and  $\mathbf{e} = (1/\sqrt{2}, 1/\sqrt{2}, 0)^T$ . Choosing  $n_c = 2$  results in a broad-band pulse

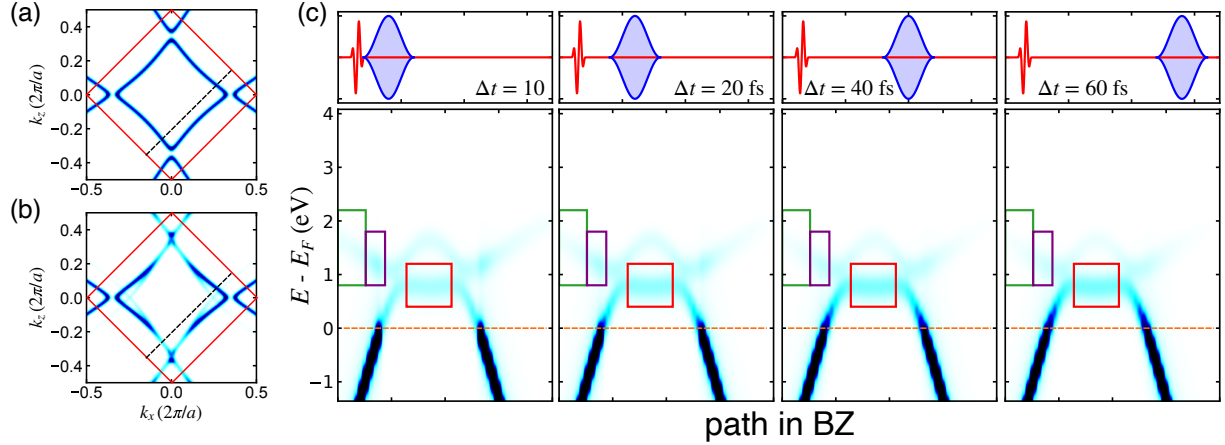

Figure S5: Fermi surface calculated from the introduced tight-binding Hamiltonian (7) for  $V_{\text{CDW}} = 0$  (a), and  $V_{\text{CDW}} = 0.2$  eV (b). The red square represents the 2D Brillouin zone for the Te plane, while the dashed line illustrates the chosen path in momentum space for which trARPES spectra are presented in (c). (c): Time-resolved photoemission spectra along the path shown in (a), (b) for  $U = 1t_{\parallel}$  and  $V_{\text{CDW}} = 0$  as function of the pump-probe delay  $\Delta t$ . The upper panels show the pump (red) and probe pulse envelope (blue).

which gives rise to a similar excited-state distribution as in the experiments (choosing  $A_0$  accordingly), which we have explicitly confirmed by comparing the experimental spectra to the simulations.

While the simulations are performed in the entire Brillouin zone, we focus on the experimentally relevant region cutting through the CDW gap. Fig. S5(a)–(b) illustrates the path in the Brillouin zone (chosen as in the experiments) along which the time-resolved photoemission spectra (10) are calculated. For the evaluation of Eq. (10) we insert the shape function

$$s(t) = \sin^2 \left( \frac{\pi(t - \Delta t)}{T_{\text{pr}}} \right), \quad \Delta t \leq t \leq \Delta t + T_{\text{pr}}, \quad (20)$$

where  $T_{\text{pr}} = 20$  fs is chosen as good compromise between energy resolution and attainable time scales.

#### 4.1 Electron-electron scattering dynamics

To investigate the thermalization dynamics in the presence e–e scattering, we simulated the dynamics including the self-energy (15) (and with the Hartree-Fock contribution). Since the time scale of e–e scattering depends on the amount of injected energy [14, 15], we calculated the absorbed energy as a function of  $A_0$  for various values of the CDW state, characterized by  $V_{\text{CDW}}$ . Comparison to experimental spectra shortly after the pulse corresponds to  $V_{\text{CDW}} \approx 0.2$  eV, which is chosen as a reference. We fix  $A_0$  to fit the excited-state carrier distribution in the experiment for the CDW phase. For other values of  $V_{\text{CDW}}$ ,  $A_0$  is determined by requiring that the same amount of energy has been absorbed.

Fig. S5(c) shows the time-resolved spectra for the metallic phase ( $V_{\text{CDW}} = 0$ ). The pump pulse promotes electrons to the upper bands, in particular in the region indicated by the green and purple boxes, which are connected to the occupied bands by the vertical transitions (see  $\Delta t = 10$  fs). Apart from

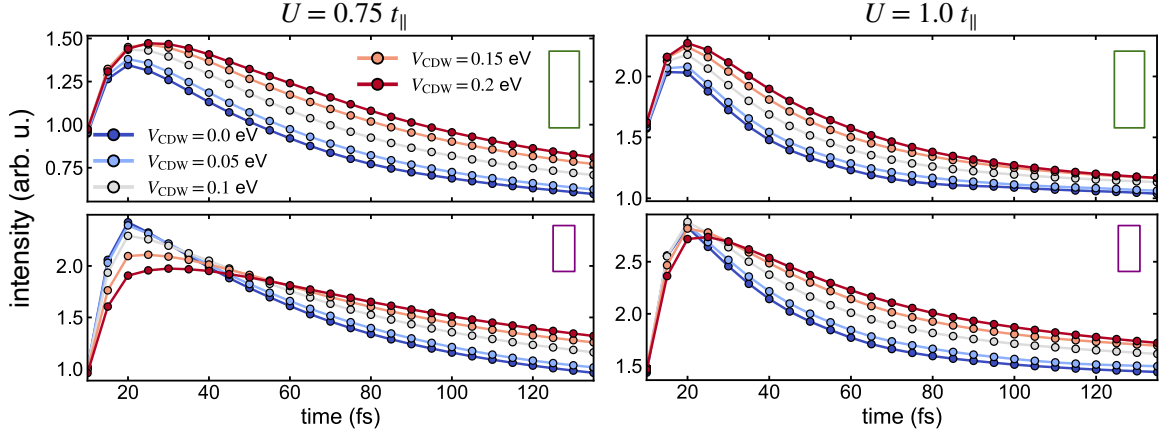

Figure S6: Integrated intensity over the relevant ROIs (illustrated by the green and the purple box in Fig. S5(c), respectively) as function of the pump-probe delay  $\Delta t$ . Left panels:  $U = 0.75 t_{||}$ , right panels:  $U = 1.0 t_{||}$ .

these resonant transitions, the occupation is broadly distributed. This is due to the short pulse and due to ultrafast e–e interactions. The latter effect gives rise to significantly increased absorption compared to the noninteracting case [10]. Furthermore, ultrafast scattering also facilitates additional intra-band transitions [9]. The time-resolved spectra for larger  $\Delta t$  show the thermalization dynamics, characterized by a relaxation towards a high-temperature thermal state. In particular, the initially sharply defined Fermi surface gets smeared as the population accumulates above the Fermi energy  $E_F$ , while the intensity in the bands at higher energy declines. While the total energy is conserved in the presence of e–e scattering only, the carriers’ mean excess energy above  $E_F$  decays.

Note that the excited-state distribution observed in the experiments is similar, albeit the presence of additional bands at  $E - E_F \approx -0.5$  eV modifies the population, specifically in the region indicated by the red boxes in Fig. S5(c). A direct comparison between theory and experiment is difficult in this region of the energy and momentum space, especially on the attainable time scales in the simulations. We will thus restrict the analysis on the region indicated by the purple and the green box in Fig. S5(c). The scattering dynamics discussed below is however generic.

For a quantitative analysis we have calculated time traces by integrating over regions in energy and momentum space, in analogy to the analysis of the experimental spectra. Fig. S6 shows the relaxation dynamics of the highly excited states for various values of the CDW parameter  $V_{CDW}$ . We also compare the dynamics for  $U = 0.75 t_{||}$  to  $U = 1.0 t_{||}$  to confirm that the observed behavior is generic. Since  $U^2$  is the scaling factor for the self-energy (15), the relaxation time scale is approximately twice as long for  $U = 0.75 t_{||}$  compared to  $U = 1.0 t_{||}$ . The qualitative behavior is very similar in both simulations. Note that, for the simulations presented in the main text,  $U = 1.0 t_{||}$  was used.

## 4.2 Effects of electron-phonon coupling

To contrast the scattering channels, we also consider electron-phonon (e–ph) coupling. As confirmed experimentally, the dominant phonon mode is an inter-plane mode perpendicular to the Te plane, with a

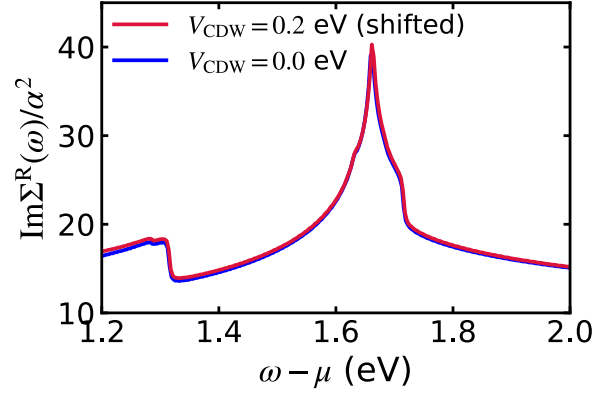

Figure S7: Imaginary part of the retarded electron-phonon self-energy  $\Sigma^{\text{e-ph,R}}(\omega)$  of the conduction band (projected onto the first BZ) for  $V_{\text{CDW}} = 0$  and  $V_{\text{CDW}} = 0.2$  eV. We shifted the frequency dependence for  $V_{\text{CDW}} = 0.2$  eV to compensate for the small shift of the conduction band upon switching on  $V_{\text{CDW}}$ . A  $N_k = 4000 \times 4000$  was required to achieve convergence.

frequency of  $\omega_{\text{ph}} \approx 15$  meV. This scenario is captured by including Holstein-type coupling:

$$\hat{H}_{\text{e-ph}} = \frac{\alpha}{\sqrt{2N}} \sum_{\mathbf{k}, \mathbf{q}} \sum_{i, \sigma} \hat{c}_{\mathbf{k}i\sigma}^\dagger \hat{c}_{\mathbf{k}-\mathbf{q}i\sigma} (\hat{b}_{\mathbf{q}} + \hat{b}_{-\mathbf{q}}^\dagger), \quad (21)$$

where  $\hat{b}_{\mathbf{q}}$  denotes the phonon annihilation operator, while  $N$  is the number of points sampling the Brillouin zone.

Here we treat the electron-phonon (e-ph) coupling within the Migdal approximation [16]:

$$\Sigma_{ij}^{\geq}(\mathbf{k}; t, t') = i\alpha^2 G_{ij}^{\text{loc}, \geq}(t, t') D_0^{\geq}(t, t'), \quad (22)$$

where  $G_{ij}^{\text{loc}}(t, t') = \frac{1}{N_k} \sum_{\mathbf{k}} G_{ij}(\mathbf{k}; t, t')$  denotes the local GF, while  $D_0(t, t')$  represents the free phonon propagator. The e-ph coupling strength is denoted by  $\alpha$ . Since we consider a single Einstein mode, the phonon propagator  $D_0^{\geq}(t, t')$  does not exhibit a momentum dependence. For this reason, the self-energy (22) is momentum independent.

To assess the effects of e-ph scattering, we calculated the retarded component of the self-energy (22)

$$\Sigma_{ij}^{\text{R}}(\omega) = \int_0^\infty dt e^{i\omega t} \left[ \Sigma_{ij}^>(t, t') - \Sigma_{ij}^<(t, t') \right]. \quad (23)$$

In Fig. S7 we compare the imaginary part for the metallic and the CDW phase over a range of  $\omega$  corresponding to the relevant conduction band. Note that the bare conduction band is shifted by 18 meV to higher energy in the CDW phase. For a one-to-one comparison we shifted the self-energy in the CDW phase in Fig. S7 accordingly. As Fig. S7 demonstrates, the self-energy of the conduction band shows practically no dependence on  $V_{\text{CDW}}$ . Hence, the relaxation dynamics for the same pulse-induced population – if only e-ph coupling is present – is identical in the metallic and the CDW phase. This is consistent with the discussion of the scattering phase space in the main text. In contrast to e-e scattering, the relaxation

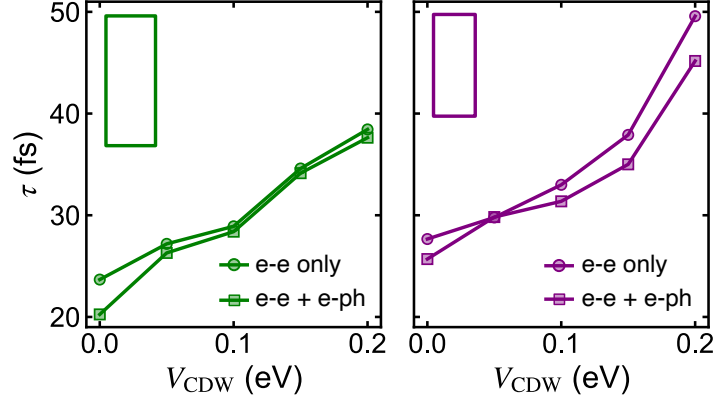

Figure S8: Relaxation time extracted in the regions of interest (analogous to Fig. 3(c) in the main text). Circles represent the case of e–e scattering only, while squares show the relaxation times for the Hubbard-Holstein model with  $\alpha = 10^{-3}$ .

of highly-excited electrons within the top band is always possible upon emitting a phonon. The presence of an electron gap at the Fermi level does not influence the probability of this process.

To confirm this picture we have performed additional GKBA simulations where we included both the e–e self-energy (15) and the e–ph self-energy (22). The simulations were carried out analogously to the case of e–e scattering only. After computing the trARPES spectrum via Eq. (10), we analyzed the ROIs as the main text and extracted the corresponding relaxation time  $\tau$ , which is shown in Fig. S8. The e–ph coupling strength can be estimated by matching the quasi-particle lifetime determined by the imaginary part of the e–ph self-energy (Fig. S7) to the long-time relaxation behavior in the experiments ( $t > 500$  fs).

In contrast to the case of e–e scattering only, in Fig. S8 we compare the extracted relaxation times with and without e–ph scattering. As Fig. S8 demonstrates, the scattering time is slightly reduced by introducing the e–ph coupling. The monotonic dependence of  $V_{\text{CDW}}$  is retained. This analysis underpins that e–ph scattering can not give rise to a significant dependence of the scattering dynamics on the CDW state.

## References

- [1] J. Maklar, Y. W. Windsor, C. W. Nicholson, M. Puppini, P. Walmsley, V. Esposito, M. Porer, J. Rittmann, D. Leuenberger, M. Kubli, M. Savoini, E. Abreu, S. L. Johnson, P. Beaud, G. Ingold, U. Staub, I. R. Fisher, R. Ernstorfer, M. Wolf, and L. Rettig, *Nat. Commun.* **12**, 2499 (2021).
- [2] H. Ding, T. Yokoya, J. C. Campuzano, T. Takahashi, M. Randeria, M. R. Norman, T. Mochiku, K. Kadowaki, and J. Giapintzakis, *Nature* **382**, 51 (1996).
- [3] J. M. Harris, Z. X. Shen, P. J. White, D. S. Marshall, M. C. Schabel, J. N. Eckstein, and I. Bozovic, *Phys. Rev. B* **54**, R15665 (1996).
- [4] A. G. Loeser, Z.-X. Shen, D. S. Dessau, D. S. Marshall, C. H. Park, P. Fournier, and A. Kapitulnik, *Science* **273**, 325 (1996).

- [5] F. Schmitt, P. S. Kirchmann, U. Bovensiepen, R. G. Moore, J.-H. Chu, D. H. Lu, L. Rettig, M. Wolf, I. R. Fisher, and Z.-X. Shen, [New J. Phys. \*\*13\*\*, 063022 \(2011\)](#).
- [6] V. Brouet, W. L. Yang, X. J. Zhou, Z. Hussain, R. G. Moore, R. He, D. H. Lu, Z. X. Shen, J. Laverock, S. B. Dugdale, N. Ru, and I. R. Fisher, [Phys. Rev. B \*\*77\*\*, 235104 \(2008\)](#).
- [7] G. Stefanucci and R. v. Leeuwen, *Nonequilibrium Many-Body Theory of Quantum Systems: A Modern Introduction* (Cambridge University Press, 2013).
- [8] J. Freericks, H. Krishnamurthy, and T. Pruschke, [Phys. Rev. Lett. \*\*102\*\*, 136401 \(2009\)](#).
- [9] M. Sentef, A. F. Kemper, B. Moritz, J. K. Freericks, Z.-X. Shen, and T. P. Devereaux, [Phys. Rev. X \*\*3\*\*, 041033 \(2013\)](#).
- [10] M. Schüler, U. De Giovannini, H. Hübener, A. Rubio, M. A. Sentef, T. P. Devereaux, and P. Werner, [Phys. Rev. X \*\*10\*\*, 041013 \(2020\)](#).
- [11] M. Schüler, J. C. Budich, and P. Werner, [Phys. Rev. B \*\*100\*\*, 041101 \(2019\)](#).
- [12] Y. Murakami, M. Schüler, S. Takayoshi, and P. Werner, [Phys. Rev. B \*\*101\*\*, 035203 \(2020\)](#).
- [13] R. Tuovinen, D. Golež, M. Eckstein, and M. A. Sentef, [Phys. Rev. B \*\*102\*\*, 115157 \(2020\)](#).
- [14] N. Tsuji and P. Werner, [Phys. Rev. B \*\*88\*\*, 165115 \(2013\)](#).
- [15] M. Schüler, Y. Murakami, and P. Werner, [Phys. Rev. B \*\*97\*\*, 155136 \(2018\)](#).
- [16] G. D. Mahan, *Many-Particle Physics* (Springer Science & Business Media, 2000).
